# Supplementary material for: Atom Interferometry with Floquet Atom Optics
Source: arXiv:2205.06965 ancillary file (2023-01-17)
Supplement: Supplementary file 1 [file Floquet_Supplemental.pdf]

# Atom Interferometry with Floquet Atom Optics: Supplemental Material

Thomas Wilkason,<sup>1,\*</sup> Megan Nantel,<sup>2,\*</sup> Jan Rudolph,<sup>1,\*</sup> Yijun Jiang (姜一君),<sup>2</sup>  
Benjamin E. Garber,<sup>1</sup> Hunter Swan,<sup>1</sup> Samuel P. Carman,<sup>1</sup> Mahiro Abe,<sup>1</sup> and Jason M. Hogan<sup>1,†</sup>

<sup>1</sup>*Department of Physics, Stanford University, Stanford, California 94305, USA*

<sup>2</sup>*Department of Applied Physics, Stanford University, Stanford, California 94305, USA*

(Dated: May 14, 2022)

## GENERALIZED $\pi$ -PULSE CONDITION

The main text makes use of solutions to the strong drive Rabi problem that allow for perfect transfer between the ground and excited states of a two-level system. Specifically, for a given detuning  $\Delta$  and Rabi coupling strength  $\Omega$ , we look for the modulation offset  $\delta = \beta - |\Delta|$  that leads to perfect state inversion after some evolution time  $t_\pi$ . Here we describe the requirements of these solutions in terms of a generalized  $\pi$ -pulse condition which applies in both the strong and weak coupling regimes.

Using Floquet's theorem, we write the time evolution operator as  $\hat{U}(t) = \hat{P}(t) e^{\frac{i}{2}\hat{\sigma}_z \Delta \epsilon t} \hat{P}^\dagger(0)$ , where  $\hat{P}(t)$  is periodic with period  $T$  and  $\Delta \epsilon$  is the quasienergy difference between the two Floquet modes [1]. In the matrix representation of  $\hat{P}(t)$  in the bare atom basis  $\{|g\rangle, |e\rangle\}$ , the columns of the matrix  $\langle i | \hat{P}(t) | j \rangle$  correspond to the two Floquet modes  $|u_\pm(t)\rangle$  with associated quasienergies  $\pm \frac{1}{2} \Delta \epsilon$ . As such,  $\hat{P}(t)$  is the unitary operator that rotates the bare atom states  $\{|g\rangle, |e\rangle\}$  to the Floquet states  $|u_\pm(t)\rangle$ . Indeed,  $\hat{P}(t)$  is the transformation that diagonalizes the Floquet Hamiltonian  $\hat{H}_F = \hat{H}(t) - i\partial_t$ . In spherical coordinates we have in general

$$\hat{P}(t) = e^{\frac{i}{2}\hat{\sigma}_z(\alpha(t)-\phi(t))} e^{-\frac{i}{2}\hat{\sigma}_y\theta(t)} e^{\frac{i}{2}\hat{\sigma}_z\phi(t)},$$

where  $\alpha(t)$ ,  $\theta(t)$ , and  $\phi(t)$  are all periodic real functions with period  $T$ . Here  $\theta(t)$  and  $\Phi(t) \equiv \phi(t) - \alpha(t)$  are the polar and azimuthal angles of the Floquet modes on the Bloch sphere. Assuming the system starts in the ground state  $|g\rangle$  at  $t = 0$ , for efficient transitions we want to maximize the amplitude of the excited state  $|e\rangle$  at some time  $t$ , which is

$$\langle e | \hat{U}(t) | g \rangle = \chi_-(t) \cos \frac{A(t)}{2} + i\chi_+(t) \sin \frac{A(t)}{2}, \quad (\text{S1})$$

where we define the pulse area as  $A(t) \equiv \int_0^t \Delta \epsilon + \dot{\phi}(t') dt'$  and  $\chi_\pm(t) \equiv \sin \left( \frac{\theta(t) \pm \theta(0)}{2} \right)$ . For an ideal  $\pi$  pulse,  $|\langle e | \hat{U} | g \rangle|$  should reach one at some time  $t = t_\pi$ . We identify the following generalized  $\pi$ -pulse conditions sufficient to achieve perfect state transfer for any coupling strength:

$$A(t_\pi) = \pi \quad (\text{S2})$$

$$\theta(t_\pi) = \pi - \theta(0) \quad (\text{S3})$$

To search for solutions that satisfy these constraints, we solve for  $\theta(t)$  and  $\phi(t)$  as well as the quasienergy difference  $\Delta \epsilon$  by diagonalizing the Floquet Hamiltonian  $\hat{H}_F$  represented in the Fourier basis. In the weak coupling limit ( $\Omega \ll |\Delta|$ ) this can be done approximately by treating the counter-rotating terms in the matrix  $\hat{H}_F$  as a perturbation. For sine-wave modulation  $\Omega(t) = \Omega_0 \cos \beta t$ , we find to leading order  $\Delta \epsilon \approx \beta + \sqrt{(\beta - |\Delta|)^2 + (\Omega_0/2)^2}$ ,  $\phi(t) \approx -\beta t$ , and  $\theta(t) \approx \theta_0$  with  $\tan \frac{\theta_0}{2} \equiv \frac{\Omega_0/2}{\delta + \Omega_g}$  and  $\Omega_g \equiv \sqrt{\delta^2 + (\Omega_0/2)^2}$ . We thus recover the usual rotating wave approximation (RWA) solution with pulse area  $A(t_\pi) \approx \Omega_g t_\pi$ . Examining the  $\theta(t)$  condition, we find in this limit  $\chi_- = 0$  and  $\chi_+ \approx \frac{\Omega_0/2}{\Omega_g}$ , which is the usual Lorentzian line shape factor in the Rabi oscillation formula that describes the energy resonance. In this limit, Eqs. S2 and S3 are decoupled and we can independently find  $\delta$  to maximize the resonance condition  $\chi_+(t)^2$ , resulting in  $\delta = 0$ . The optimum  $t_\pi$  then follows immediately from the area constraint.

In the strong coupling regime ( $\Omega \sim |\Delta|$ ), these two constraints for the generalized  $\pi$ -pulse condition become coupled and must be solved for simultaneously. We numerically diagonalize the Floquet Hamiltonian  $\hat{H}_F$  after truncating to a sufficiently large finite matrix to minimize error. Figure S1 shows the pulse area  $A(t)$  and the resonance factor  $\chi_+(t)^2$  as a function of the modulation frequency  $\beta$  for sine-wave modulation for several values of  $t_\pi$ . When  $\Omega \sim |\Delta|$ , the strong drive dynamics causes  $\chi_+(t)^2$  to differ markedly from a Lorentzian and to depend strongly on the pulse time. This is a consequence of the fact that in the strong drive limit, the Floquet modes periodically exchange energy with

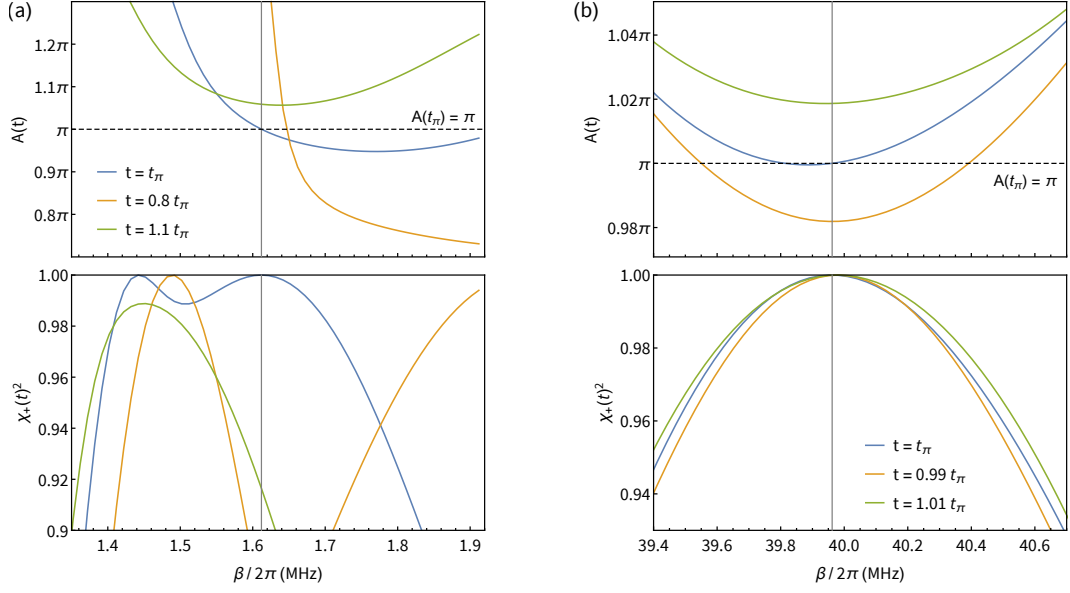

FIG. S1. (a) Generalized  $\pi$ -pulse conditions in the strong coupling regime ( $\Omega \sim |\Delta|$ ) for sine-wave modulation  $\Omega(t) = \Omega_0 \cos \beta t$  with  $\Delta = 2\pi \times 2.0$  MHz and  $\Omega_0 = 2\pi \times 5.0$  MHz. Pulse area  $A(t)$  (upper panel) and amplitude factor  $\chi_+(t)^2$  (lower panel) as a function of modulation frequency  $\beta$  for three choices of the pulse time: optimal time  $t_\pi = 237.9$  ns (blue),  $0.8 t_\pi$  (orange), and  $1.1 t_\pi$  (green). The gray line shows the optimal solution at  $\beta = 2\pi \times 1.612$  MHz. (b) Generalized  $\pi$ -pulse conditions in the weak coupling regime ( $\Omega \ll |\Delta|$ ) with  $\Delta = 2\pi \times 40.0$  MHz and  $\Omega_0 = 2\pi \times 5.0$  MHz for three different pulse durations:  $t_\pi = 200.1$  ns (blue),  $0.99 t_\pi$  (orange), and  $1.01 t_\pi$  (green). The optimum modulation frequency in this case is found to be  $\beta = 2\pi \times 39.962$  MHz (gray line), which approaches the RWA solution  $\beta \approx |\Delta|$  as expected in this limit. The amplitude factor  $\chi_+(t)^2$  is here approximately Lorentzian (lower panel) with a peak that is almost independent of  $t_\pi$ , while the area condition (upper panel) shows an approximate linear dependence on  $t_\pi$  as expected.

the drive as described in the main text. Likewise, the area constraint  $A(t)$  exhibits a non-trivial  $\beta$  dependence that it inherits from the quasienergy spectrum, and it now has a nonlinear dependence on  $t_\pi$ . These features of the strong drive case are a manifestation of the time dependence of the Floquet modes, which replace the static dressed states that appear in the well-known weak drive solution.

### ANALYTIC SOLUTION OF PULSE PARAMETERS FOR SQUARE-WAVE MODULATION

In the case of a square-wave Floquet pulse, the amplitude of the Rabi coupling  $\Omega(t)$  is constant during each half period  $T/2$ , and the state precesses at a constant rate  $\sqrt{\Omega_0^2 + \Delta^2}$  about the torque vector  $(\Omega(t), 0, \Delta)$ . As  $\Omega(t)$  evolves, the torque vector alternates between  $(+\Omega_0, 0, \Delta)$  and  $(-\Omega_0, 0, \Delta)$ , resulting in a state trajectory that consists of a series of circular arcs on the Bloch sphere. As described in the main text, finding the optimal pulse parameters in this case reduces to a purely geometric problem of determining the intersections of a series of cones determined by the torque vector during each half-period segment.

We assume the system is initially in the excited state, corresponding to the south pole of the Bloch sphere, and that the goal is to reach the ground state (north pole) with perfect transfer efficiency. The number of half-periods  $n$  required to reach the target state depends on the angle  $\alpha$  that the torque vector makes with the  $z$ -axis, given by  $\tan \alpha \equiv \frac{\Omega_0}{|\Delta|}$ . In general, a solution with  $n$  cones exists for detuning in the range  $\cot\left(\frac{\pi}{2(n-1)}\right) \leq \frac{|\Delta|}{\Omega_0} \leq \cot\left(\frac{\pi}{2n}\right)$ . Equivalently, in terms of  $\alpha$  we have the requirement

$$\frac{\pi}{2n} \leq \alpha \leq \frac{\pi}{2(n-1)} \quad (\text{S4})$$

for a solution to exist with  $n$  cones. Note that since we restrict ourselves to the case of periodic modulation, where the duration of each segment of  $\Omega(t)$  is a fixed length  $T/2$ , the angle swept out by the state vector as it precesses about each of the first  $(n-1)$  cones will be a constant value  $\Delta\theta_n$ . In terms of this angle, the solution for the modulation

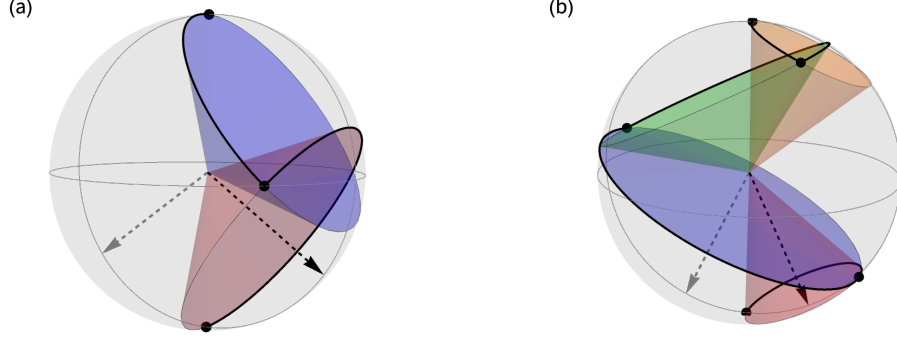

FIG. S2. (a) Bloch sphere evolution for square-wave modulation with  $\alpha = \frac{3\pi}{10} \approx 0.942$  illustrating a geometric solution consisting of  $n = 2$  cones. The initial torque vector is shown as a black dashed arrow and the torque vector during the second half-period is a gray dashed arrow. The state evolution is shown in black, tracing around the base of the two cones (red and then blue), while the initial and final states are shown as black dots at the bottom and top, respectively. (b) Bloch sphere evolution with  $\alpha = \frac{17\pi}{120} \approx 0.445$  illustrating a solution with  $n = 4$  cones. The state precesses along the base of the red, blue, green, and then orange cone, in that order. As in (a), the torque vector toggles between the black and gray dashed arrows on alternating half-periods, and these arrows serve as the axes of all the cones.

frequency  $\beta = 2\pi/T$  in the case of  $n$  cones is given by

$$\beta_n = 2\pi \frac{\sqrt{\Omega_0^2 + \Delta^2}}{2\Delta\theta_n} \quad (\text{S5})$$

In a typical solution, the system will reach the target state at some time  $t_\pi$  that is not equal to an integer number of half-periods  $T/2$ . Instead, during the last segment of the state trajectory, only a fraction of the half-period is required to reach the target state. Consequently, the angle of precession around the last cone will be some smaller angle  $\Delta\phi_n$ . In terms of these two precession angles  $\Delta\theta_n$  and  $\Delta\phi_n$ , the required total pulse duration in the case of  $n$  cones is given by

$$t_\pi = \frac{(n-1)\Delta\theta_n + \Delta\phi_n}{\sqrt{\Omega_0^2 + \Delta^2}} \quad (\text{S6})$$

where once again the integer  $n$  is determined by the angle  $\alpha$  of the torque vector at a given detuning and Rabi frequency. The Bloch sphere evolution for two example solutions is shown in Fig. S2.

For the range  $\frac{\pi}{4} \leq \alpha \leq \frac{\pi}{2}$ , solutions exist with  $n = 2$  and the following precession angles:

$$\Delta\theta_2 = \pi + 2 \sec^{-1}(\sqrt{2} \sin \alpha) \quad (\text{S7})$$

$$\Delta\phi_2 = \pi - 2 \sec^{-1}(\sqrt{2} \sin \alpha) \quad (\text{S8})$$

These correspond to the solutions for  $\beta$  and  $t_\pi$  given in the main text. Note that the case  $n = 2$  is special in that the total precession angle is  $\Delta\theta_2 + \Delta\phi_2 = 2\pi$ , which is independent of  $\alpha$ . This implies that for detunings in the range  $0 \leq |\Delta| \leq \Omega_0$ , the total precession angle of the state is always  $2\pi$ . This is the same as in common composite pulse sequences such as the well-known  $\frac{\pi}{2} - \pi_{90^\circ} - \frac{\pi}{2}$  pulse, which also requires  $2\pi$  of pulse area. However, since the Floquet pulse precession rate is the generalized Rabi frequency  $\sqrt{\Omega_0^2 + \Delta^2}$  instead of  $\Omega_0$ , the Floquet pulse requires less time.

For the range  $\frac{\pi}{6} \leq \alpha \leq \frac{\pi}{4}$ , we have solutions with  $n = 3$  given by

$$\Delta\theta_3 = 2\pi - \cos^{-1} \left( \frac{\sin 3\alpha - \sqrt{7 \cos^2 \alpha + 1}}{4 \sin \alpha \cos^2 \alpha} \right) \quad (\text{S9})$$

$$\Delta\phi_3 = \cos^{-1} \left( \frac{\sin \alpha + \sqrt{7 \cos^2 \alpha + 1}}{4 \sin \alpha \cos^2 \alpha} - \cot^2 \alpha \right) \quad (\text{S10})$$

and for the range  $\frac{\pi}{8} \leq \alpha \leq \frac{\pi}{6}$ , we have solutions with  $n = 4$  given by

$$\Delta\theta_4 = 2\pi - 2\sin^{-1}\left(\sqrt{\frac{1+3r_4(r_4+1)}{12r_4\cos^2\alpha}}\right) \quad (\text{S11})$$

$$\Delta\phi_4 = 2\tan^{-1}\left(\frac{\tan\frac{\Delta\theta_4}{2}(3-4\cos^2\alpha\sin^2\frac{\Delta\theta_4}{2})}{4\cos^2\alpha\sin^2\frac{\Delta\theta_4}{2}-1}\right) \quad (\text{S12})$$

where  $r_4 \equiv \left(\cot^2(\alpha) + \sqrt{\frac{26}{27} + \cos(2\alpha)\csc^4(\alpha)}\right)^{1/3}$ . Finally, for the range  $\frac{\pi}{10} \leq \alpha \leq \frac{\pi}{8}$ , we have solutions with  $n = 5$  given by

$$\Delta\theta_5 = \pi + \cos^{-1}\left(\frac{5+\eta+\sqrt{19-\eta^2+\frac{2}{\eta}}}{8\cos^2\alpha}-1\right) \quad (\text{S13})$$

$$\Delta\phi_5 = 2\tan^{-1}\left(\frac{\frac{1}{4}(\cos 4\alpha + \cot^2\frac{\Delta\theta_5}{2})\sec^4\alpha\tan\frac{\Delta\theta_5}{2}-\sin\Delta\theta_5}{\cos\Delta\theta_5+\tan^2\alpha}\right) \quad (\text{S14})$$

where

$$\eta \equiv \sqrt{\frac{19}{3}-\frac{4}{3}\left(\frac{43\cos^2\alpha-19-r_5^2}{r_5\sin\alpha}\right)} \quad (\text{S15})$$

$$r_5 \equiv \left((82-253\cos^2\alpha)\sin\alpha + \sqrt{27}\sqrt{574\cos^6\alpha+4\cos^4\alpha-61\cos^2\alpha-5}\right)^{1/3} \quad (\text{S16})$$

Another special case is when the angle  $\alpha$  lies on the boundary of the ranges specified by Eq. S4. For  $\alpha = \frac{\pi}{2n}$  with integer  $n$ , the cones are all tangent and each one intersects with the next at a single point. In this case, the precession angle during each half-period is exactly  $\pi$ , so we have  $\Delta\theta_n = \pi$  and  $\Delta\phi_n = \pi$ . The modulation frequency then becomes  $\beta_n = \Omega_0 \csc \alpha = \Omega_0 \csc \frac{\pi}{2n}$ . In the large detuning limit,  $\alpha \ll 1$  and  $n \gg 1$  so we have  $\beta_n \approx |\Delta|$ . This corresponds to the limit  $\delta = \beta - |\Delta| \approx 0$  given in the main text for the resonance condition in the weak coupling limit. Likewise, for  $\alpha = \frac{\pi}{2n}$  the pulse time is  $t_\pi = \frac{n\pi}{\Omega_0} \sin \frac{\pi}{2n}$ . In the weak coupling limit,  $n \gg 1$  and we have  $t_\pi \approx \frac{\pi}{2} \frac{\pi}{\Omega_0} = \frac{\pi}{2} t_0$ , which matches the asymptotic limit given in the main text for square-wave modulation.

## ASYMPTOTIC LIMITS OF THE PULSE DURATION

As shown in the main text, the Floquet pulse duration in the weak coupling limit ( $\Omega \ll |\Delta|$ ) converges to  $t_\pi = 2t_0$  for sine-wave and  $t_\pi = \frac{\pi}{2}t_0$  for square-wave modulation. This result can be understood by considering the pulse envelope function  $\Omega(t)$  in the frequency domain. For periodic drive at frequency  $\beta = 2\pi/T$ , the Fourier expansion is

$$\Omega(t) = \sum_{m=-\infty}^{\infty} \Omega_m e^{im\beta t} \quad (\text{S17})$$

where  $\Omega_m$  is the Fourier coefficient at frequency  $m\beta$ . As noted above, the optimum modulation frequency converges to  $\beta \approx \Delta$  in the weak coupling limit. When this occurs, the  $m = 1$  frequency component is directly on resonance with the atomic transition shifted by  $\Delta$ . Since the other Fourier components are all far detuned in this limit, the dynamics are completely determined by the  $\Omega_1$  component. This situation corresponds to the rotating wave approximation (RWA) limit, where the  $\Omega_1$  term is the co-rotating frequency component and the counter-rotating term  $\Omega_{-1}$  (and all other terms detuned by multiples of  $\beta$ ) can be neglected. As a result, the pulse duration in the weak coupling limit is simply determined by the Rabi oscillation time associated with the  $\Omega_1$  Fourier amplitude. For square-wave modulation, we have from the Fourier expansion  $\Omega_1 = \frac{2}{\pi}\Omega_0$ , resulting in  $t_\pi = \frac{\pi}{\Omega_1} = \frac{\pi}{2}t_0$  with  $t_0 \equiv \frac{\pi}{\Omega_0}$ . For sine-wave modulation,  $\Omega(t) = \Omega_0 \cos \beta t$  implies  $\Omega_1 = \frac{1}{2}\Omega_0$  and  $t_\pi = 2t_0$ .

The asymptotic pulse duration for sine-wave modulation with a given available optical power depends on the method used to generate  $\Omega(t)$ . In our case, we use an acousto-optic modulator (AOM) to amplitude modulate the light, resulting in an optical power of  $P(t) = P_0 \cos^2 \beta t$ , where  $P_0$  is the available power emitted by the laser. Since the

average power sent to the atoms is  $\langle P(t) \rangle = \frac{P_0}{2}$ , half of the available power is wasted, and the resulting Floquet pulses require a longer duration than the square-wave Floquet pulses. In principle, it is possible to use the available power more efficiently and reduce the pulse time. For example, the light could be split on a 50/50 beamsplitter, then the two halves could be frequency shifted up and down by  $\pm\beta$  respectively, and finally recombined on some frequency-selective optic. Directly synthesizing the sine-wave modulated Fourier spectrum in this way would result in an optical power delivered to the atoms of  $P(t) = 2P_0 \cos^2 \beta t$ , where the average power is now  $\langle P(t) \rangle = P_0$  as desired. In this ideal case, we would have Fourier coefficient  $\Omega_1 = \frac{1}{\sqrt{2}}\Omega_0$ , and the asymptotic pulse duration in the weak coupling limit would instead be  $t_\pi = \sqrt{2}t_0$  for sine-wave modulation. Therefore, the idealized sine-wave modulation would result in shorter duration pulses than square-wave modulation. This is expected because square-wave modulation wastes optical power in the higher harmonics of its Fourier expansion compared to ideal sine-wave modulation.

## COMPENSATION OF SELF-PHASE MODULATION

Our use of amplitude-modulated light in optical fibers results in intensity-dependent phase shifts arising from self-phase modulation (SPM) [2]. For example, in the case of a sine-wave modulated Floquet pulse, the applied pulse envelope is  $\bar{\Omega}(t) = \cos \beta t$  and the associated intensity in the fiber is  $I(t) = I_0 \bar{\Omega}(t)^2 = I_0 \cos^2 \beta t$ , where  $I_0$  is the peak intensity. This leads to an anomalous phase shift after exiting the fiber of  $\frac{2\pi}{\lambda} n_2 I(t) L$ , where  $n_2$  is the second-order nonlinear index of refraction and  $L$  is the length of the fiber. This spurious phase modulation breaks the symmetric evolution on the Bloch sphere that is associated with amplitude modulation, as described in the main text. To avoid this, we add a compensatory phase to the initial rf waveform used to drive the AOM, ensuring that the delivered light pulses remain purely amplitude modulated when they reach the atoms. In particular, the compensated drive voltage applied to the AOM has the form

$$\begin{aligned} W(t) &= W_0 \bar{\Omega}(t) \sin [\omega_0 t + \alpha_c I(t)] \\ &= W_0 \bar{\Omega}(t) \sin [\omega_0 t + \alpha_c I_0 \bar{\Omega}(t)^2] \end{aligned} \quad (\text{S18})$$

where  $\alpha_c$  is the effective nonlinear SPM coefficient for our system,  $\omega_0 = 2\pi \times 190$  MHz is the AOM carrier frequency, and the amplitude  $W_0$  is empirically determined by the rf power needed to maximize AOM diffraction efficiency. Note that we use a 2 GSa/s arbitrary function generator (AFG) to directly synthesize  $W(t)$  (both carrier and envelope), which allows us to easily incorporate the desired SPM compensation phase into the rf waveform.

To empirically determine the coefficient  $\alpha_c$ , we characterize the SPM by interfering the light after the fiber with unshifted light from the 0<sup>th</sup> order of the AOM. This results in a beat note at the AOM carrier frequency  $\omega_0$ , modulated by the pulse envelope  $\bar{\Omega}(t)$ . We high-pass filter the data to remove components of the beat note proportional to  $\bar{\Omega}(t)^2$  and then fit the remaining interference term to a model given by

$$V(t) = V_0 \bar{\Omega}(t) \sin [\omega_0 t + \phi_0 + \alpha_{\text{NL}} I(t)] \quad (\text{S19})$$

where  $\alpha_{\text{NL}}$  is the inferred SPM coefficient, and  $\phi_0$  and  $V_0$  are additional fit parameters.

We measure the optical beat note at different values of SPM compensation coefficient  $\alpha_c$  and extract the fitted value of  $\alpha_{\text{NL}}$  in each case. Figure S3 shows the inferred residual nonlinear phase coefficient as a function of  $\alpha_c$ . We find a compensation coefficient of  $\alpha_c = 4$  minimizes SPM. This compensation phase is used to generate the waveforms for all of the sine-wave Floquet pulses. Measurements of the atomic state time evolution confirm that this value of  $\alpha_c$  corresponds to symmetric evolution for positive and negative detunings, as expected for pure AM. Finally, we note that this particular optimum value of  $\alpha_c$  is specific to the beam intensity, and must be re-characterized at different operating Rabi frequencies.

## PULSE EFFICIENCY PROBABILITY DENSITY FUNCTION

Here we derive the probability density function (PDF) for the measured pulse efficiency for square-wave Floquet pulses used as a fitting function in the main text. The noise model includes pulse area noise due to shot-to-shot intensity noise as well as additive detection noise.

Since square-wave Floquet pulses are piecewise constant, the evolution during each half-period  $T/2$  is simple Rabi oscillations at the given detuning. For example, during the first half-period we expect the excited state population to be of the form  $P_e(t) = \eta \sin^2 \frac{A(t)}{2} = \frac{\eta}{2} - \frac{\eta}{2} \cos A(t)$ , where  $A(t)$  is the pulse area at time  $t$  and  $\eta$  is the peak population.

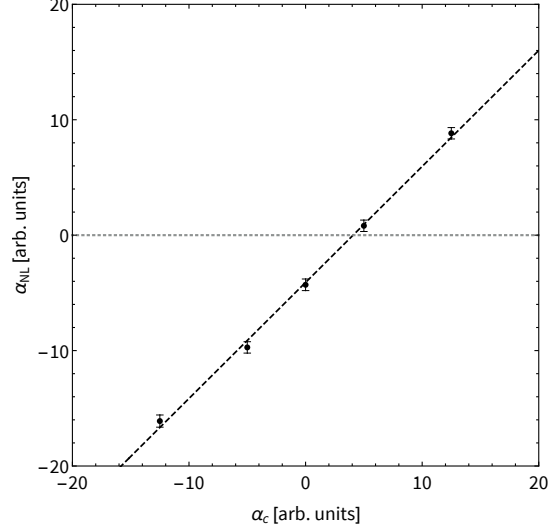

FIG. S3. Measurement of the residual nonlinear phase coefficient  $\alpha_{NL}$  as a function of the compensation phase coefficient  $\alpha_c$ . The intersection of the fitted line (black, dashed) with  $\alpha_{NL} = 0$  (gray, dotted) determines the necessary compensatory phase to use in the rf waveform of the AFG.

During subsequent half-periods, the initial conditions are different but the sinusoidal character of the solution is the same. Generally, the solution during the  $n$ th half-period may be written  $P_e(t) = b - \frac{c}{2} \cos A(t)$ , where  $b$  and  $c$  are constants that depend on the initial conditions of the half-period. For the purpose of this model, we treat  $b$  and  $c$  as fitting parameters that describe the population evolution in the vicinity of the last half-period of the Floquet pulse, the point of maximum transfer efficiency.

To characterize the pulse efficiency, we make repeated measurements of the atom population  $y$  after a Floquet pulse. This set of measured populations  $\{y_i\}$  is considered to be a sampling of some continuous random variable  $Y$ . On any given shot, the population follows from the formula for  $P_e$  above, and so has the form

$$y = h(a, b) = b - \frac{c}{2} \cos a \quad (\text{S20})$$

where  $a$  is the pulse area on that shot. As indicated by  $y = h(a, b)$ , the random variable  $Y$  is assumed to be a function of two random variables. To model area noise, we assume  $a$  is drawn from a continuous random variable  $A$ , while for additive detection noise,  $b$  is sampled from a continuous random variable  $B$ . We assume these noise sources are independent and that they can each be approximated by Gaussian PDFs. Specifically, for random variables  $A$  and  $B$  we have PDFs

$$f_A(a) = \frac{1}{\sqrt{2\pi}\delta a} e^{-\frac{1}{2}\left(\frac{a-\bar{a}}{\delta a}\right)^2} \quad (\text{S21})$$

$$f_B(b) = \frac{1}{\sqrt{2\pi}\delta b} e^{-\frac{1}{2}\left(\frac{b-\bar{b}}{\delta b}\right)^2} \quad (\text{S22})$$

where  $\delta a$  and  $\delta b$  are the widths and  $\bar{a}$  and  $\bar{b}$  are the offsets of their respective PDFs.

To find the PDF  $f_Y(y)$  for  $y$ , we first find the cumulative distribution function (CDF)  $F_Y(y)$ , since this is the same as the joint CDF for  $A$  and  $B$ . Specifically, we have

$$F_Y(y) = P(Y \leq y) = P(h(a, b) \leq y) = F_{AB}(\{a, b\} : h(a, b) \leq y) \quad (\text{S23})$$

where  $P(Y \leq y)$  is the probability that the random variable  $Y$  is less than  $y$ . This is equal to the probability of getting a value of  $a$  and  $b$  in a range such that  $h(a, b) \leq y$ .

Since  $A$  and  $B$  are independent, their joint PDF is  $f_{AB}(a, b) = f_A(a)f_B(b)$ . The joint CDF is therefore

$$F_{AB}(y) = \int_{h(a, b) \leq y} f_{AB}(a, b) da db \quad (\text{S24})$$

When specifying the bounds of integration here, we restrict the range of the population to  $0 \leq y \leq 1$  and assume the pulse area lies in the range  $0 \leq a \leq 2\pi$ . Although the Gaussian PDF for  $A$  is actually unbounded, in practice the area noise is sufficiently small ( $\delta a \ll 2\pi$ ) and concentrated around  $\bar{a} = \pi$  that this is a good approximation. The joint CDF (for  $y > 1 - \frac{c}{2}$ ) is then

$$\begin{aligned}
F_{AB}(y) = & \int_{\frac{\pi}{2}}^{\frac{3\pi}{2}} \int_0^{y + \frac{c}{2} \cos a} f_{AB}(a, b) db da \\
& + \int_{\arccos(\frac{1-y}{c/2})}^{\frac{\pi}{2}} \int_{\frac{c}{2} \cos a}^{y + \frac{c}{2} \cos a} f_{AB}(a, b) db da + \int_{\frac{3\pi}{2}}^{2\pi - \arccos(\frac{1-y}{c/2})} \int_{\frac{c}{2} \cos a}^{y + \frac{c}{2} \cos a} f_{AB}(a, b) db da \\
& + \int_0^{\arccos(\frac{1-y}{c/2})} \int_{\frac{c}{2} \cos a}^1 f_{AB}(a, b) db da + \int_{2\pi - \arccos(\frac{1-y}{c/2})}^{2\pi} \int_{\frac{c}{2} \cos a}^1 f_{AB}(a, b) db da
\end{aligned} \tag{S25}$$

To find the PDF we then differentiate since  $f_Y(y) = \frac{dF_Y(y)}{dy} = \frac{dF_{AB}(y)}{dy}$ , resulting in

$$f_Y(y) = \int_{\arccos(\frac{1-y}{c/2})}^{2\pi - \arccos(\frac{1-y}{c/2})} f_A(a) f_B(y + \frac{c}{2} \cos a) da \tag{S26}$$

It is convenient to transform this result with the substitution  $p \equiv \frac{c}{2} \cos a$ ,

$$f_Y(y) = \int_{-\frac{c}{2}}^{1-y} \frac{f_B(y+p)}{\sqrt{(c/2)^2 - p^2}} \left( f_A\left(\arccos\left(\frac{p}{c/2}\right)\right) + f_A\left(2\pi - \arccos\left(\frac{p}{c/2}\right)\right) \right) dp \tag{S27}$$

which takes the form of a convolution of  $f_B$  over the area noise PDF, as well as the factor  $\sqrt{(c/2)^2 - p^2}$  which also appears in the population PDF used in atom interference experiments [3].

---

\* These authors contributed equally to this work.

† [hogan@stanford.edu](mailto:hogan@stanford.edu)

- [1] J. H. Shirley, Solution of the schrödinger equation with a hamiltonian periodic in time, *Phys. Rev.* **138**, B979 (1965).
- [2] R. H. Stolen and C. Lin, Self-phase-modulation in silica optical fibers, *Phys. Rev. A* **17**, 1448 (1978).
- [3] R. Geiger, V. Ménoret, G. Stern, N. Zahzam, P. Cheinet, B. Battelier, A. Villing, F. Moron, M. Lours, Y. Bidel, *et al.*, Detecting inertial effects with airborne matter-wave interferometry, *Nature Communications* **2**, 474 (2011).
